# Supplementary material for: Improving Evaluation of Debiasing in Image Classification
Source: arXiv:2206.03680 source file (2023-04-14)
Supplement: Supplementary file 1 [file supple_tab_cmnist.tex]

\begin{table}[t!]
\centering
\scalebox{0.63}{
\begin{tabular}{cccccccccccccccc}
\toprule
\multirow{2.5}{*}{Dataset} 
& \multirow{2.5}{*}{Ratio (\%)} 
&
& Vanilla
& LNL
& EnD
& HEX
& ReBias
& Softcon
& LfF
& DisEnt
& NSS
& JTT
& SSA
& EIIL
& GroupDRO
\\
\cmidrule{4-16}
&&
& \textcolor{black}{\boldxmark} \textcolor{black}{\boldxmark}
& \textcolor{black}{\boldxmark} \textcolor{black}{\boldcheckmark}
& \textcolor{black}{\boldcheckmark} \textcolor{black}{\boldcheckmark}
& \textcolor{black}{\boldcheckmark} \textcolor{black}{\boldcheckmark}
& \textcolor{black}{\boldxmark} \textcolor{black}{\boldcheckmark}
& \textcolor{black}{\boldxmark} \textcolor{black}{\boldcheckmark}
& \textcolor{black}{\boldxmark} \textcolor{black}{\boldxmark}
& \textcolor{black}{\boldxmark} \textcolor{black}{\boldxmark}
& \textcolor{black}{\boldxmark} \textcolor{black}{\boldxmark}
& \textcolor{black}{\boldxmark} \textcolor{black}{\boldxmark}
& \textcolor{black}{\boldxmark} \textcolor{black}{$\triangle$}
& \textcolor{black}{\boldxmark} \textcolor{black}{\boldxmark}
& \textcolor{black}{\boldcheckmark} \textcolor{black}{\boldcheckmark}
\\
\midrule
\multirow{5}{*}{\makecell{MLP}} 
& 0.5 & & 34.61 & 36.69 & 34.54 & 24.58 & 21.62 & 31.29 & 62.01 & 59.99 & \textbf{66.71} & 63.61 & - & - & - \\ & 1.0 & & 49.87 & 57.87 & 46.83 & 39.80 & 31.01 & 47.66 & 76.17 & 73.30 & \textbf{77.94} & 68.75 & - & - & - \\ & 2.0 & & 66.84 & 70.71 & 61.35 & 50.76 & 47.04 & 60.79 & 82.63 & 76.86 & \textbf{82.98} & 79.76 & - & - & - \\ & 5.0 & & 81.56 & 81.50 & 78.56 & 79.58 & 73.24 & 79.46 & 86.43 & 84.05 & \textbf{88.74} & 84.37 & - & - & - \\ & 20.0 & & \textbf{92.77} & 92.22 & 90.73 & 91.02 & 91.68 & 89.57 & 90.76 & 91.97 & 91.32 & 86.96 & - & - & - \\
\midrule
\multirow{5}{*}{\makecell{Simple Conv}} 
& 0.5 & & 73.45 & 76.28 & 73.10 & 13.21 & 54.07 & 78.29 & 89.54 & 83.69 & \textbf{92.27} & 84.49 & - & - & - \\ & 1.0 & & 87.57 & 87.64 & 85.39 & 15.58 & 75.13 & 88.22 & 90.74 & 87.77 & \textbf{93.29} & 91.52 & - & - & - \\ & 2.0 & & 93.07 & 92.03 & 91.15 & 42.71 & 88.32 & 95.84 & 95.79 & 91.35 & \textbf{96.05} & 95.64 & - & - & - \\ & 5.0 & & 95.65 & 96.02 & 95.35 & 66.36 & 95.11 & 97.61 & 96.25 & 95.88 & 97.62 & \textbf{98.02} & - & - & - \\ & 20.0 & & 98.07 & 98.42 & 98.20 & 92.95 & 98.11 & \textbf{98.90} & 97.54 & 98.06 & 98.15 & 98.79 & - & - & - \ 
\bottomrule
\end{tabular}
}
\caption{Image classification accuracy evaluated on tests sets with model selection after certain iterations. The \textit{cross} and \textit{check} marks denote whether each algorithm requires 1) bias labels during training and 2) prior knowledge on bias types in that order. The best results are marked in bold.}
\label{tab:main1}
\end{table}
